# Supplementary material for: CAMMARL: Conformal Action Modeling in Multi Agent Reinforcement Learning
Source: arXiv:2306.11128 source file (2024-02-09)
Supplement: Supplementary file 1 [file supplementary.tex]

\documentclass{article} % For LaTeX2e
\usepackage{iclr2024_conference,times}

% Optional math commands from https://github.com/goodfeli/dlbook_notation.
\input{math_commands.tex}

\usepackage{hyperref}
\usepackage{url}% Include other packages here, before hyperref.
\usepackage{graphicx}
\usepackage{amsmath}
\usepackage{amssymb}
\usepackage{booktabs}
\usepackage{subcaption}
\usepackage{algorithm} 
\usepackage{algpseudocode} 
\usepackage{lipsum}
\usepackage{bbm} 
\usepackage{soul}

% Support for easy cross-referencing
\usepackage[capitalize]{cleveref}
\crefname{section}{Sec.}{Secs.}
\Crefname{section}{Section}{Sections}
\Crefname{table}{Table}{Tables}
\crefname{table}{Tab.}{Tabs.}

\newcommand{\algo}{\textsc{cammarl}}

\usepackage[acronym]{glossaries}
\glsdisablehyper 
\newacronym{cn}{CN}{cooperative navigation} 
\newacronym{lbf}{LBF}{level-based foraging} 
\newacronym{marl}{MARL}{multi-agent reinforcement learning} 

\begin{document}

%%%%%%%%% TITLE - PLEASE UPDATE
\title{Supplementary \\ \algo: Conformal Action Modeling in \\Multi Agent Reinforcement Learning}

\author{%
Nikunj Gupta\thanks{Corresponding author.} $^{123}$ \quad Samira Ebrahimi Kahou $^{124}$ \\
$^1$Mila Quebec AI Institute \quad $^2$ÉTS Montréal \quad $^3$New York University \quad $^4$CIFAR AI Chair\\
\texttt{nikunj.gupta@nyu.edu, samira.ebrahimi.kahou@gmail.com}
}
\maketitle

\label{sec:appendix}
\input{chapters/10_appendix}
%------------------------------------------------------------------------

\bibliography{main}
\bibliographystyle{iclr2024_conference}

\end{document}
